# Supplementary material for: Measurement of Born cross section of $e^+e^-\to\Sigma^0\bar{\Sigma}^0$ at $\sqrt{s} = 3.50-4.95$ GeV
Source: arXiv:2412.20305 source file (2025-03-15)
Supplement: Supplementary file 1 [file supplement.pdf]

# Supplement Material for "Measurement of Born cross section of $e^+e^- \to \Sigma^0\bar{\Sigma}^0$ at $\sqrt{s} = 3.5 - 4.9$ GeV"

TABLE I. The $e^+e^- \to \Sigma^0\bar{\Sigma}^0$ Born cross section $\sigma^B$ and effective form factor $G_{\rm eff}(s)$ for thirty-two energy points between 3.50 and 4.95 GeV. The values in the brackets are the corresponding upper limits at 90% C.L. The first uncertainties are statistical, and the second ones are systematic uncertainties. The $\sqrt{s}$ is the $e^+e^-$ CM energy [1, 2]. The $\int \mathcal{L}dt$ is the integrated luminosity of each data set [3–5], the vacuum polarization correction factor $\frac{1}{|1-\Pi|^2}$, the products of the ISR correction factor and the detection efficiency $\epsilon(1+\delta)$ . The $N_{\rm S}$ is the number of events in the signal region, $N_{\rm bkg}$ is the number of background events scaled by sideband region, $N_{\rm obs}$ is the number of observed events by subtracting the backgrounds with the uncertainty calculated by the Rolke's method [6] (the number of signal events for the upper limit with the consideration of systematic uncertainty estimated based on Rolke's method [6]). The $S$ is statistical significance.

| $\sqrt{s}$ (GeV) | $\int \mathcal{L}dt$ (pb$^{-1}$) | $\frac{1}{\lvert 1-\Pi\rvert^2}$ | $\epsilon(1+\delta)$ | $N_{\rm S}$ | $N_{\rm bkg}$ | $N_{\rm obs}$ | $\sigma^B$ (fb) | $G_{\rm eff}(s)$ ($\times 10^{-3}$) | $S(\sigma)$ |
|---|---|---|---|---|---|---|---|---|---|
| 3.51 | 405.4 | 1.045 | 0.163 | 17 | 0.5 | $16.5^{+5.0}_{-3.3}$ | $583^{+175}_{-117}\pm28$ | $9.6^{+1.4}_{-1.0}\pm0.2$ | 4.0 |
| 3.58154 | 85.7 | 1.039 | 0.168 | 3 | 0.5 | $2.5^{+2.6}_{-0.9}$ ($<6.9$) | $407^{+420}_{-149}\pm20$ ($<1119$) | $8.1^{+4.2}_{-1.5}\pm0.2$ ($<13.5$) | 1.4 |
| 3.65 | 410.0 | 1.021 | 0.168 | 4 | 0.5 | $3.5^{+2.8}_{-1.2}$ ($<8.3$) | $121^{+99}_{-41}\pm6$ ($<288$) | $4.5^{+1.8}_{-0.8}\pm0.1$ ($<6.9$) | 1.8 |
| 3.67016 | 84.7 | 1.000 | 0.166 | 3 | 0.0 | $3.0^{+2.1}_{-1.4}$ ($<6.9$) | $518^{+359}_{-245}\pm25$ ($<1186$) | $9.3^{+3.2}_{-2.2}\pm0.2$ ($<14.1$) | 1.7 |
| 3.773 | 2931.8 | 1.056 | 0.168 | 73 | 9.5 | $63.5^{+9.4}_{-7.7}$ | $297^{+44}_{-36}\pm14$ | $7.2^{+0.6}_{-0.5}\pm0.2$ | 7.4 |
| 3.87131 | 110.3 | 1.051 | 0.174 | 1 | 0.0 | $1.0^{+1.4}_{-0.7}$ ($<3.7$) | $121^{+164}_{-85}\pm6$ ($<444$) | $4.7^{+3.2}_{-1.6}\pm0.1$ ($<9.0$) | 1.0 |
| 4.00762 | 482.0 | 1.044 | 0.175 | 7 | 0.5 | $6.5^{+3.5}_{-1.8}$ ($<12.4$) | $180^{+97}_{-50}\pm8$ ($<344$) | $5.9^{+1.6}_{-0.8}\pm0.1$ ($<8.2$) | 2.5 |
| 4.12848 | 401.5 | 1.052 | 0.162 | 2 | 0.5 | $1.5^{+2.3}_{-0.6}$ ($<5.3$) | $53^{+80}_{-21}\pm3$ ($<189$) | $3.3^{+2.5}_{-0.7}\pm0.1$ ($<6.2$) | 1.1 |
| 4.15744 | 408.7 | 1.053 | 0.165 | 2 | 0.5 | $1.5^{+2.3}_{-0.6}$ ($<5.3$) | $51^{+77}_{-21}\pm2$ ($<183$) | $3.3^{+2.5}_{-0.7}\pm0.1$ ($<6.2$) | 1.1 |
| 4.1783 | 3189.0 | 1.054 | 0.169 | 12 | 1.8 | $10.3^{+4.6}_{-2.4}$ | $44^{+20}_{-10}\pm2$ | $3.0^{+0.7}_{-0.4}\pm0.1$ | 3.0 |
| 4.1989 | 526.0 | 1.056 | 0.170 | 3 | 0.0 | $3.0^{+2.1}_{-1.4}$ ($<6.9$) | $78^{+54}_{-37}\pm4$ ($<177$) | $4.1^{+1.4}_{-1.0}\pm0.1$ ($<6.1$) | 1.7 |
| 4.2092 | 517.1 | 1.057 | 0.166 | 1 | 0.3 | $0.8^{+1.6}_{-0.4}$ ($<3.7$) | $20^{+43}_{-12}\pm1$ ($<99$) | $2.1^{+2.2}_{-0.6}\pm0.0$ ($<4.6$) | 0.8 |
| 4.22626 | 514.6 | 1.057 | 0.164 | 3 | 0.0 | $3.0^{+2.1}_{-1.4}$ ($<6.9$) | $82^{+57}_{-39}\pm4$ ($<188$) | $4.2^{+1.5}_{-1.0}\pm0.1$ ($<6.3$) | 1.7 |
| 4.23 | 1100.9 | 1.056 | 0.171 | 3 | 0.3 | $2.8^{+2.3}_{-1.2}$ ($<6.9$) | $34^{+29}_{-14}\pm2$ ($<84$) | $2.7^{+1.1}_{-0.6}\pm0.1$ ($<4.3$) | 1.6 |
| 4.2357 | 530.3 | 1.056 | 0.170 | 1 | 0.8 | $0.3^{+2.1}_{-0.1}$ ($<3.7$) | $6^{+54}_{-1}\pm0$ ($<94$) | $1.2^{+5.0}_{-0.1}\pm0.0$ ($<4.5$) | 0.3 |
| 4.2438 | 538.1 | 1.056 | 0.170 | 2 | 0.0 | $2.0^{+1.8}_{-1.1}$ ($<5.3$) | $50^{+44}_{-28}\pm2$ ($<135$) | $3.3^{+1.5}_{-0.9}\pm0.1$ ($<5.4$) | 1.4 |
| 4.25797 | 828.4 | 1.054 | 0.170 | 1 | -0.3 | $1.3^{+1.1}_{-0.9}$ ($<3.7$) | $21^{+18}_{-16}\pm1$ ($<60$) | $2.1^{+0.9}_{-0.8}\pm0.0$ ($<3.6$) | 1.3 |
| 4.2668 | 531.1 | 1.053 | 0.170 | 5 | 0.5 | $4.5^{+3.1}_{-1.4}$ ($<9.7$) | $115^{+79}_{-36}\pm5$ ($<249$) | $5.0^{+1.7}_{-0.8}\pm0.1$ ($<7.4$) | 2.0 |
| 4.2777 | 175.7 | 1.053 | 0.164 | 1 | 0.0 | $1.0^{+1.4}_{-0.7}$ ($<3.7$) | $80^{+109}_{-56}\pm4$ ($<294$) | $4.2^{+2.8}_{-1.5}\pm0.1$ ($<8.0$) | 1.0 |
| 4.28788 | 502.4 | 1.053 | 0.158 | 1 | 0.0 | $1.0^{+1.4}_{-0.7}$ ($<3.7$) | $29^{+40}_{-20}\pm1$ ($<107$) | $2.5^{+1.7}_{-0.9}\pm0.1$ ($<4.9$) | 1.0 |
| 4.31205 | 501.2 | 1.052 | 0.158 | 1 | 0.0 | $1.0^{+1.4}_{-0.7}$ ($<3.7$) | $29^{+40}_{-20}\pm1$ ($<107$) | $2.6^{+1.7}_{-0.9}\pm0.1$ ($<4.9$) | 1.0 |
| 4.33739 | 505.0 | 1.051 | 0.161 | 2 | 0.0 | $2.0^{+1.8}_{-1.1}$ ($<5.3$) | $57^{+50}_{-31}\pm3$ ($<152$) | $3.6^{+1.6}_{-1.0}\pm0.1$ ($<5.8$) | 1.4 |
| 4.35826 | 544.0 | 1.051 | 0.169 | 1 | 0.5 | $0.5^{+1.9}_{-0.2}$ ($<3.7$) | $13^{+47}_{-5}\pm1$ ($<92$) | $1.7^{+3.1}_{-0.3}\pm0.0$ ($<4.6$) | 0.5 |
| 4.37737 | 522.7 | 1.051 | 0.158 | 3 | 0.0 | $3.0^{+2.1}_{-1.4}$ ($<6.9$) | $84^{+58}_{-40}\pm4$ ($<193$) | $4.4^{+1.5}_{-1.0}\pm0.1$ ($<6.6$) | 1.7 |
| 4.39645 | 507.8 | 1.051 | 0.159 | 1 | 0.5 | $0.5^{+1.9}_{-0.2}$ ($<3.7$) | $14^{+54}_{-6}\pm1$ ($<106$) | $1.8^{+3.4}_{-0.4}\pm0.0$ ($<4.9$) | 0.5 |
| 4.41558 | 1090.7 | 1.052 | 0.168 | 1 | 0.8 | $0.3^{+2.1}_{-0.1}$ ($<3.7$) | $3^{+27}_{-1}\pm0$ ($<46$) | $0.9^{+3.6}_{-0.1}\pm0.0$ ($<3.3$) | 0.3 |
| 4.43624 | 569.9 | 1.054 | 0.159 | 1 | 0.0 | $1.0^{+1.4}_{-0.7}$ ($<3.7$) | $26^{+35}_{-18}\pm1$ ($<94$) | $2.4^{+1.7}_{-0.9}\pm0.1$ ($<4.7$) | 1.0 |
| 4.59953 | 586.9 | 1.055 | 0.159 | 1 | 0.0 | $1.0^{+1.4}_{-0.7}$ ($<3.7$) | $25^{+34}_{-17}\pm1$ ($<91$) | $2.5^{+1.7}_{-0.9}\pm0.1$ ($<4.8$) | 1.0 |
| 4.612 | 103.6 | 1.055 | 0.146 | 1 | 0.0 | $1.0^{+1.4}_{-0.7}$ ($<3.7$) | $152^{+207}_{-106}\pm7$ ($<559$) | $6.2^{+4.2}_{-2.2}\pm0.1$ ($<11.9$) | 1.0 |
| 4.66124 | 529.4 | 1.054 | 0.140 | 1 | 0.0 | $1.0^{+1.4}_{-0.7}$ ($<3.7$) | $31^{+42}_{-22}\pm1$ ($<114$) | $2.8^{+1.9}_{-1.0}\pm0.1$ ($<5.4$) | 1.0 |
| 4.68192 | 1667.4 | 1.054 | 0.140 | 1 | 0.0 | $1.0^{+1.4}_{-0.7}$ ($<3.7$) | $10^{+13}_{-7}\pm0$ ($<36$) | $1.6^{+1.1}_{-0.6}\pm0.0$ ($<3.1$) | 1.0 |
| 4.78054 | 511.5 | 1.055 | 0.149 | 1 | 0.0 | $1.0^{+1.4}_{-0.7}$ ($<3.7$) | $30^{+41}_{-21}\pm1$ ($<111$) | $2.9^{+1.9}_{-1.0}\pm0.1$ ($<5.5$) | 1.0 |


[1] M. Ablikim *et al.* (BESIII Collaboration), *Chin. Phys. C* **40**, 063001 (2016).
[2] M. Ablikim *et al.* (BESIII Collaboration), *Chin. Phys. C* **45**, 103001 (2021).
[3] M. Ablikim *et al.* (BESIII Collaboration), *Chin. Phys. C* **39**, 093001 (2015).
[4] M. Ablikim *et al.* (BESIII Collaboration), *Chin. Phys. C* **46**, 113002 (2022).
[5] M. Ablikim *et al.* (BESIII Collaboration), *Chin. Phys. C* **46**, 113003 (2022).
[6] J. Lundberg, J. Conrad, W. Rolke, and A. Lopez, *Comput. Phys. Commun.* **181**, 683-686 (2010).

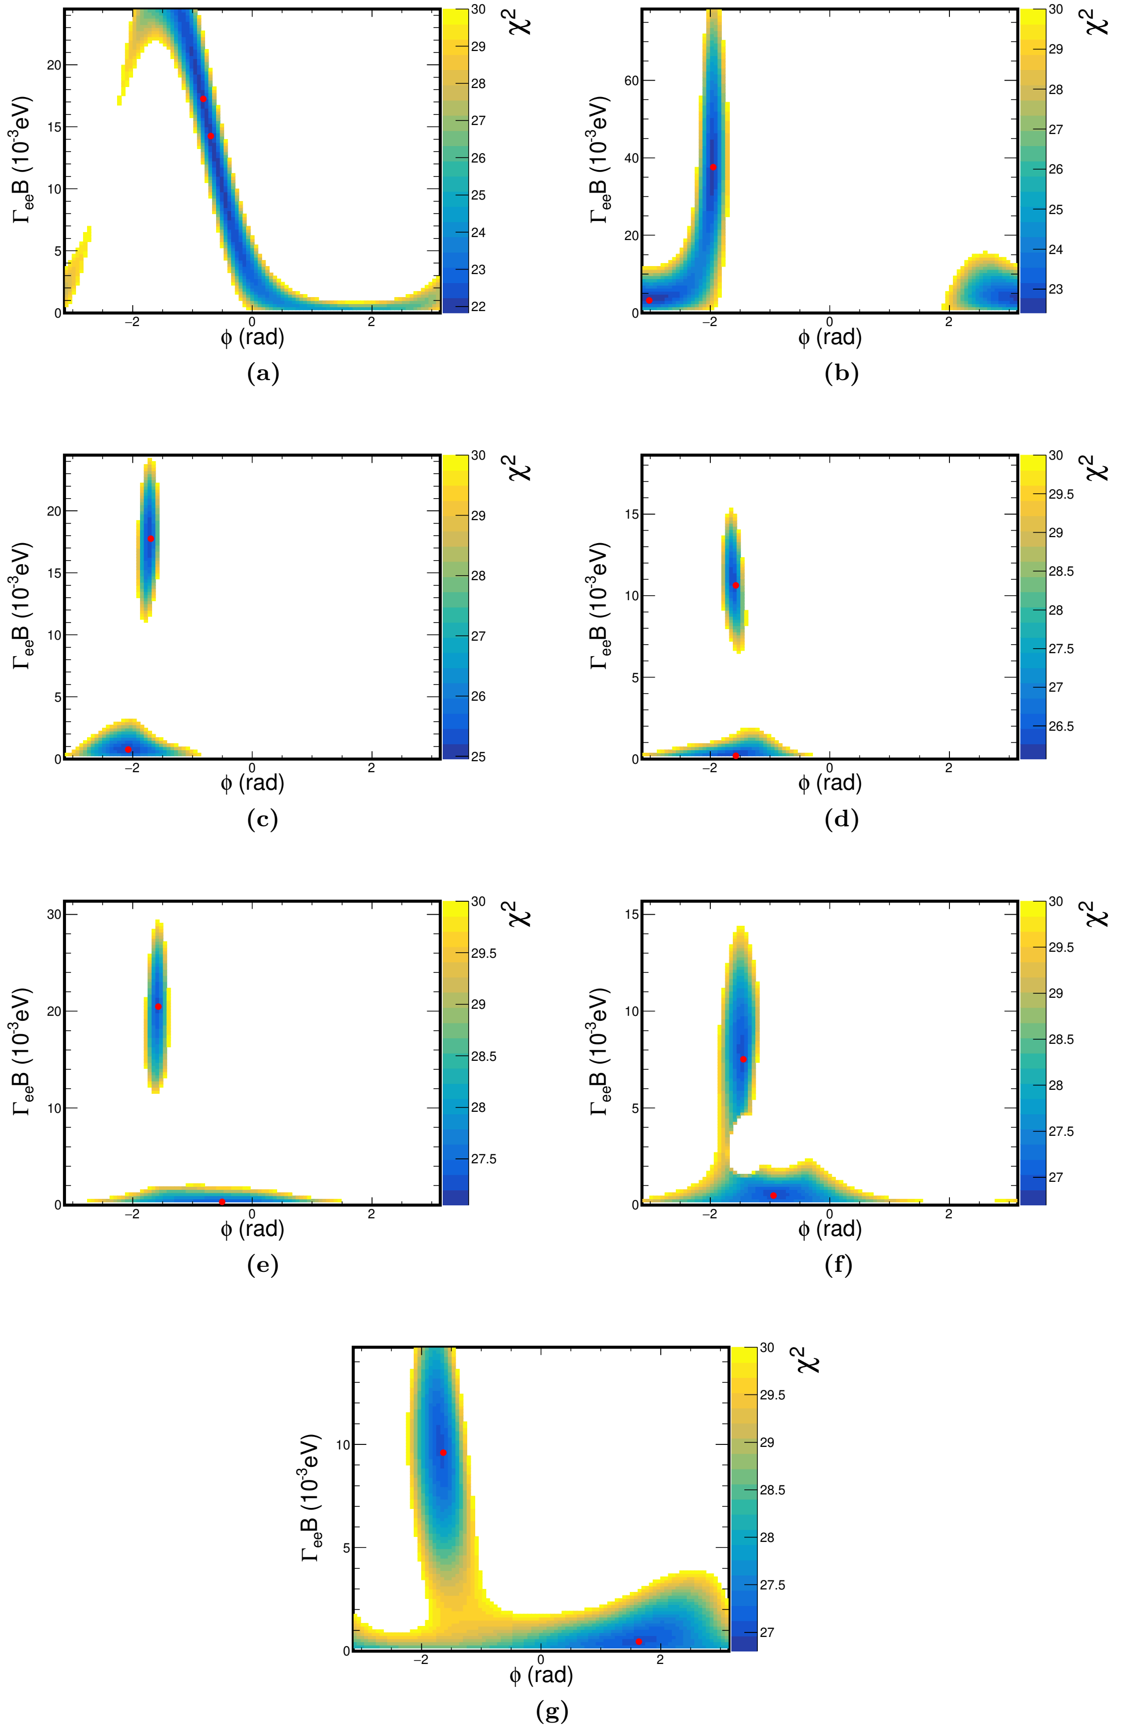


FIG. 1. The $\chi^2$ distribution versus the products of branching fraction and electronic partial width, and the relative phase $\phi$ for the resonances $\psi(3770)$ (a), $\psi(4040)$ (b), $\psi(4160)$ (c), $\psi(4230)$ (d), $\psi(4360)$ (e), $\psi(4415)$ (f) or $\psi(4660)$ (g) decaying into the $\Sigma^0\bar{\Sigma}^0$. In the figure, the red dots stands for the solution.
